# Supplementary material for: Cell division and death inhibit glassy behaviour of confluent tissues
Source: arXiv:1610.09340 ancillary file (2017-04-17)
Supplement: Supplementary file 1 [file SuppMatt.pdf]

# Supplementary material for: Cell division and death inhibit glassy behaviour of confluent tissues

## A. Influence of the division rate $d_0$

We consider again our system where the only source of activity is cell division and apoptosis. Cell division is a density dependent mechanism with division rate (Eq. 3 in the main text)

$$d = d_0 \left(1 - \frac{z}{z_{max}}\right).$$

We investigate the influence of the bare division rate $d_0$ on the steady state of the system for two attractive force strengths $\epsilon = 0$ and $\epsilon = 0.15$. The results are shown in Fig. 1. As can be seen, the overall state of the system does not change significantly with $d_0$, except at very high $d_0$ where the division time scale competes with the elastic time scale (see below).

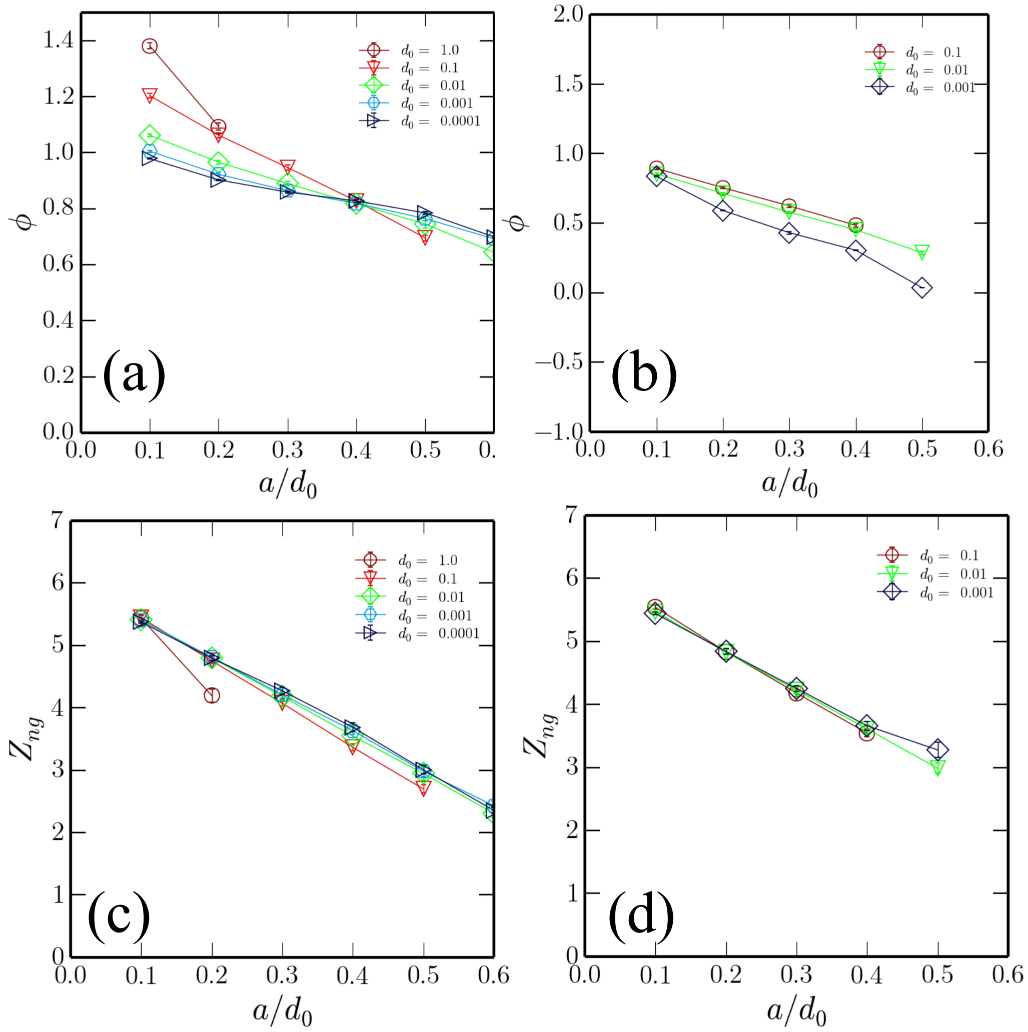


Figure 1: Influence of the bare division rate $d_0$ on the packing fraction $\Phi$ (a-b) and mean contact number $Z_{\rm ng}$ (c-d) as a function of $a/d_0$. Panel (a-c) $\epsilon = 0$ and (b-d) 0.15.

## B. Finize size effects - absorbing transition

We investigate how the system size influences the location of the *gas - absorbed* phase boundary line $\Phi = 0$. We choose a system at $(a/d_0 = 0.5, \epsilon = 0.15)$, which is just within the gas phase for a very large system with $L = 240$. We then monitor the evolution of the packing fraction $\Phi$ when we decrease the system size; the results are presented in Fig. 2. We observe that, as expected, density fluctuations play a major role for small systems. For $L < 25$ the fluctuations of the packing fraction are sufficient to remove all the cells, leading to the absorbing empty state in a first passage dynamics. Figure 3 shows the variance of the packing fraction Var($\Phi$) as function of system size. As can be seen, for small system sizes the fluctuations are comparable to $\Phi$, making any colony die out. Further work is needed to explore this effect in more detail.

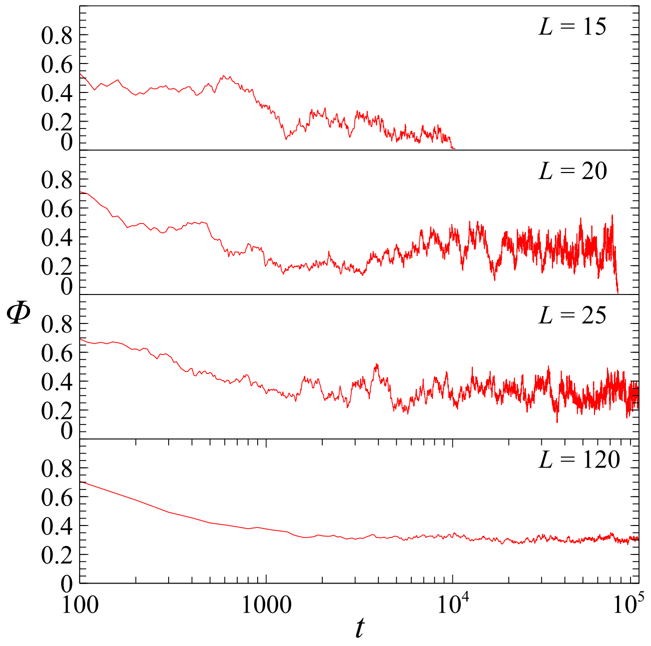


Figure 2: Influence of the system size on the packing fraction $\Phi$ for $a/d_0 = 0.5$ and $\epsilon = 0.15$.

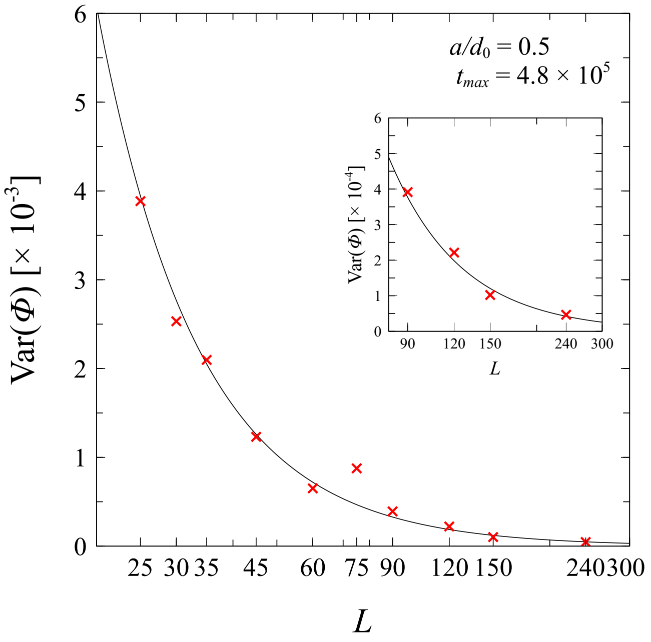


Figure 3: Variance of the packing fraction Var($\Phi$) as a function of the system size $L$. We use the same set of parameters as in Fig. 2; the maximum simulation time $t_{max}$ is indicated on the figure.

## C. Finize size effects - self-melting state

We test the influence of the system length $L$ on the dynamics of the system by using a fixed $d_0 = 0.01$, with a division rate $a/d_0 = 0.003$, and a bit higher fraction of tracer particles (5%) to improve statistics at small $L$. For the mean square displacement, there is virtually no dependence on the system size, while the self-intermediate scattering function shows a delayed fluidisation for small $L \leq 30$, but no effects for larger $L$.

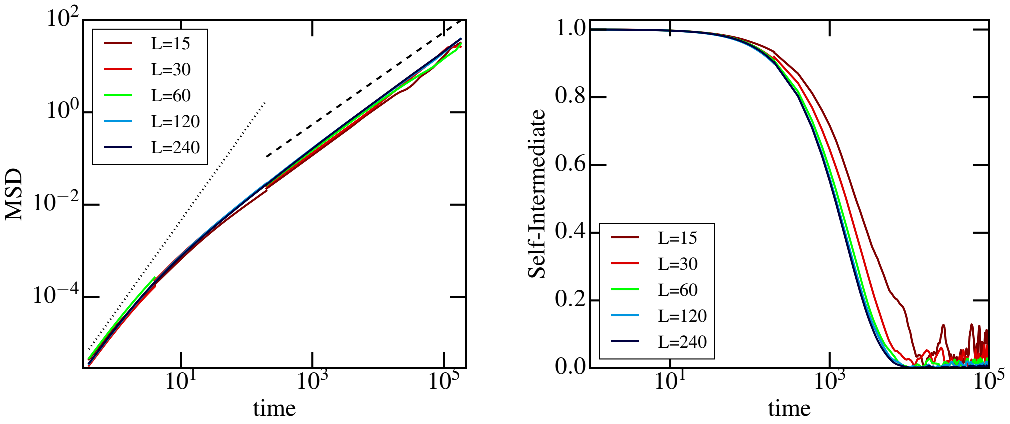


Figure 4: Influence of system size $L$ on the confluent dynamics. Left: Mean square displacement. Right: Self-Intermediate scattering function. All runs were performed at $k = 1$, $a/d_0 = 0.003$, $d_0 = 0.01$ and $\epsilon = 0.15$.

## D. Influence of the elastic time scale

In the equations of motion $\partial_t \mathbf{r}_i = \mu \mathbf{F}_i$ (Eq. 2 of the main text), the mobility $\mu$ sets the time scale of the diffusive dynamics due to particle motion. Taking the form of the potential into account, mobility and elastic constant $k$ form a single time scale $\tau_{el} = 1/\mu k$. Here, we investigate the influence of $\tau_{el}$ on the slow dynamics in the confluent phase.

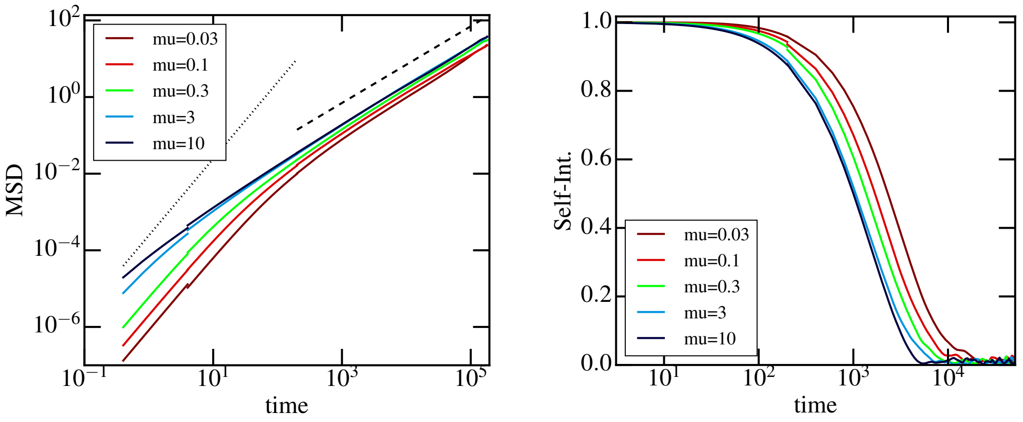


Figure 5: Influence of elastic time scale $1/\mu k$ on the confluent dynamics. Left: Mean square displacement. Right: Self-Intermediate scattering function. All runs were performed at $k = 1$, $a/d_0 = 0.01$, $d_0 = 0.003$ and $\epsilon = 0.15$.

We find a nuanced picture. At short time scales (MSD plot), the influence of $\tau_{el}$ is pronounced: for low values of $\mu$, i.e. large $\tau_{el}$, the system takes a longer time to switch from ballistic to diffusive behaviour. This confirms that the relevant time scale in the MSD is *not* set by the inverse division rate $1/a$. The curves also do not rescale with a simple power of $\tau_{el}$, pointing towards a subtler interaction of elastic and division time scales for this crossover. At longer time scales, the relaxation time scale in the Self-intermediate function is only slightly influenced by $\tau_{el}$, with larger $\mu$ leading to a faster decay, but only by about a factor of 3 over more than two orders of magnitude of change in $\tau_{el}$.

# E. GPU-Parallel Implementation

Is well known that Molecular Dynamics (MD) simulation is a highly parallelizable numerical method; implementations of MD are packages like for example LAMMPS, AMBER and GROMACS. Following these examples, we have built our own parallel MD code on GPU (NVIDIA CUDA). In contrast to LAMMPS, for example, our in-house code is specifically designed to introduce different sources of activity into the system (cell division, cell death and self propelled velocities). The general workflow of the code is shown in algorithm 1. All our routines are fully implemented on the GPU, so that there are no transfers between DEVICE-HOST during the MD execution. The only routines executed by the host (colored in blue) are those required by the user in order to save data. It is worth mentioning that these operations require data transfer between the DEVICE and the HOST, see the red colored text.

Our CUDA kernels are moderately optimized, trying to keep aligned and coalesced memory access, and avoiding threads divergence and atomic functions. Further optimizations are still possible, but there are diminishing returns since at some point they will obfuscate the code for a negligible speedup. As defensive programming techniques we use assertions, and each routine is independently tested before implementation. We do not use heavy database implementations and/or post processing packages: In most cases the output of our simulation is already the final result. Finally, we used external imaging routines for visualization, testing and presentation purposes.

**Algorithm 1:** Typical Simulation Scheme

```
(0) Give atoms initial positions and velocities;
for Simulation time do
    (1) Predict next atom positions:
        (a) Get Forces;
        (b) Move Atoms and Update Velocities;
        (c) Apply Boundary Conditions;
        (c*) Apply Lees-Edwards boundary conditions during force-shear simulations;
    (2) Cell Functions:
        (a) Cell death;
        (b) Cell division;
    (3) Build neighbours:
    if (2) or atoms move too far then
            (a) Build the linked-list;
            (b) Using (a) build the neighbour list of each atom;
    (4) Analysis:
    if Simulation time then
            (a) Standard properties: pressure, density, etc.;
            (b) Transport properties: Mean square displacement etc.;
            (c) Transfer (a) and (b) to the host (CPU);
            (d) Save (a) (b);
    (5) Save Configurations:
    if Simulation time then
            (a) Transfer atom properties to the host (CPU);
            (b) Save (a);
```
